# Supplementary material for: Weighted Information Filtering, Smoothing, and Out-of-Sequence Measurement Processing
Source: arXiv:2009.02659 source file (2020-09-06)
Supplement: Supplementary file 1 [file appendix.tex]

\section{Appendix}
\label{appendix}
\subsection{Proof of Theorem~\ref{theorem:batch}}\label{appendix:batch}
Setting to zero the gradient of~\eqref{Eq:problem:WLS} with respect to $x_k$  we obtain
\[
\sum_{\ell\in\mathcal{L}}A_{\ell,k}^TH_\ell^TW_{\ell,k}R_\ell^{-1}W_{\ell,k}^T(H_\ell(A_{\ell,k}x_k+C_{\ell,k}u_{\ell,k})-y_\ell)=0.
\]
Solving for $x_k$ yields~\eqref{Eq:batch:estimator}.
\subsection{Proof of Theorem~\ref{theorem:covariance}}\label{appendix:covariance}
Let
\begin{align}
\Sigma_k&\triangleq\paren{\sum_{\ell\in\mathcal{L}}A_{\ell,k}^TH_\ell^TW_{\ell,k}R_\ell^{-1}W_{\ell,k}^TH_\ell A_{\ell,k}}\\
\Psi_{\ell,k}&\triangleq A_{\ell,k}^TH_\ell^TW_{\ell,k}R_\ell^{-1}W_{\ell,k}^T
\end{align}
and consider the covariance of the estimator~\eqref{Eq:batch:estimator}
\begin{align}\non
P_k
&=\cov\left(\Sigma_k^{-1}\sum_{\ell\in\mathcal{L}}\Psi_{\ell,k}(y_\ell-H_\ell C_{\ell,k}u_{\ell,k})\right)\\\non
&=\Sigma_k^{-1}\paren{\sum_{\ell\in\mathcal{L}}\Psi_{\ell,k}{W}_{\ell,k}^{-T}R_\ell{W}_{\ell,k}^{-1}\Psi_{\ell,k}^T}\Sigma_k^{-T}.
\end{align}
Cancelling out appropriate terms and their inverses~\eqref{Eq:batch:covariance} follows.
\subsection{Proof of Theorem~\ref{theorem:recursive}}\label{appendix:recursive}
Consider the inverse of the covariance computed in batch form~\eqref{Eq:batch:covariance}
\begin{align}\non%\label{App:covariance:recursive}
P_k^{-1}&=\sum_{\ell=1}^kA_{\ell,k}^TH_\ell^TW_{\ell,k}R_\ell^{-1}W_{\ell,k}^TH_\ell A_{\ell,k}\\\label{Eq:covariance:recursive:proof}
&=\sum_{\ell=1}^{k-1}A_{\ell,k}^TH_\ell^TW_{\ell,k}R_\ell^{-1}W_{\ell,k}^TH_\ell A_{\ell,k}
+H_k^TR_k^{-1}H_k,
\end{align}
where we used the fact that $A_{k,k}=I$ as well as the assumption~\eqref{Eq:recursive:W:equal}. Using the fact that $A_{\ell,k}=A_{\ell,k-1}A_{k-1,k}$ as well as the assumption~\eqref{Eq:recursive:W:telescopic} the result for the covariance follows.
%&=\sum_{\ell=1}^{k-1}(A_{\ell,k-1}A_{k-1,k})^TH_\ell^TW_{k,\ell}R_\ell^{-1}W_{k,\ell}^TH_\ell(A_{\ell,k-1}A_{k-1,k})\\
%&\qquad+H_\ell^TR_\ell^{-1}H_\ell\\
%\end{align}
We utilize this result to prove the expression for $\hat{x}_k$. Consider the batch formulation first
%\begin{align}\non
%\hat{x}_k
%&=P_k\sum_{\ell=1}^kA_{\ell,k}^TH_\ell^TW_{\ell,k}R_\ell^{-1}W_{\ell,k}^T(y_\ell-H_\ell C_{\ell,k}u_{\ell,k})\\\label{Eq:estimate:recursive:proof1}
%&=P_k\Big(\sum_{\ell=1}^{k-1}A_{\ell,k}^TH_\ell^TW_{\ell,k}^2R_\ell^{-1}(y_\ell-H_\ell C_{\ell,k}u_{\ell,k})
%+H_k^TR_k^{-1}y_k\Big).
%\end{align}
\begin{align}\non
\hat{x}_k
&=P_k\sum_{\ell=1}^kA_{\ell,k}^TH_\ell^TW_{\ell,k}R_\ell^{-1}W_{\ell,k}^Ty_\ell\\\label{Eq:estimate:recursive:proof1}
&=P_k\Big(\sum_{\ell=1}^{k-1}A_{\ell,k}^TH_\ell^TW_{\ell,k}^2R_\ell^{-1}y_\ell+H_k^TR_k^{-1}y_k\Big).
\end{align}
Consider the summation
%\begin{align}\non
%&\sum_{\ell=1}^{k-1}A_{\ell,k}^TH_\ell^TW_{\ell,k}^2R_\ell^{-1}(y_\ell-H_\ell C_{\ell,k}u_{\ell,k})\\\non
%&\,=A_{k-1,k}^TW_{k-1,k}^2\sum_{\ell=1}^{k-1}A_{\ell,k-1}^TH_\ell^TW_{\ell,k-1}^2R_\ell^{-1}(y_\ell-H_\ell C_{\ell,k}u_{\ell,k}).
%\end{align}
\begin{align}\non
&\sum_{\ell=1}^{k-1}A_{\ell,k}^TH_\ell^TW_{\ell,k}^2R_\ell^{-1}y_\ell\\\non
&\qquad=A_{k-1,k}^TW_{k-1,k}^2\sum_{\ell=1}^{k-1}A_{\ell,k-1}^TH_\ell^TW_{\ell,k-1}^2R_\ell^{-1}y_\ell.
\end{align}
%It is easy to see that
%\[
%C_{\ell,k}u_{\ell,k}=A_{\ell,k-1}C_{k-1,k}u_{k-1,k}+C_{\ell,k-1}u_{\ell,k-1},
%\]
%which renders the above summation as follows
%\begin{align}\nonumber
%&\sum_{\ell=1}^{k-1}A_{\ell,k}^TH_\ell^TW_{\ell,k}^2R_\ell^{-1}(y_\ell-H_\ell C_{\ell,k}u_{\ell,k})\\\non
%&\quad=A_{k-1,k}^TW_{k-1,k}^2\sum_{\ell=1}^{k-1}A_{\ell,k-1}^TH_\ell^TW_{\ell,k-1}^2R_\ell^{-1}\\\non
%&\qquad\times(y_\ell-H_\ell (A_{\ell,k-1}C_{k-1,k}u_{k-1,k}+C_{\ell,k-1}u_{\ell,k-1})).
%\end{align}
%The latter becomes, using~\eqref{Eq:batch:estimator} and~\eqref{Eq:batch:covariance},
%\begin{align}\nonumber
%&\sum_{\ell=1}^{k-1}A_{\ell,k}^TH_\ell^TW_{\ell,k}^2R_\ell^{-1}(y_\ell-H_\ell C_{\ell,k}u_{\ell,k})\\\non
%&\quad=A_{k-1,k}^TW_{k-1,k}^2P_{k-1}^{-1}\hat{x}_{k-1}\\\non
%&\qquad\qquad-A_{k-1,k}^TW_{k-1,k}^2P_{k-1}^{-1}C_{k,k-1}u_{k,k-1}.
%%\\\non &\quad=A_{k-1,k}^TW_{k-1,k}^2P_{k-1}^{-1}(\hat{x}_{k-1}-C_{k,k-1}u_{k,k-1}).
%\end{align}
Using~\eqref{Eq:batch:estimator} and~\eqref{Eq:batch:covariance} the latter becomes
\begin{align}
&\sum_{\ell=1}^{k-1}A_{\ell,k}^TH_\ell^TW_{\ell,k}^2R_\ell^{-1}y_\ell
=A_{k-1,k}^TW_{k-1,k}^2P_{k-1}^{-1}\hat{x}_{k-1}.
%\\\non &\quad=A_{k-1,k}^TW_{k-1,k}^2P_{k-1}^{-1}(\hat{x}_{k-1}-C_{k,k-1}u_{k,k-1}).
\end{align}
Plugging this result in~\eqref{Eq:estimate:recursive:proof1} completes the proof.

\subsection{Proof of Theorem~\ref{theorem:efficient}}\label{appendix:efficient}
The unbiasedness follows trivially by substituting~\eqref{Eq:problem:state} in~\eqref{Eq:problem:measurement}, plugging the result in~\eqref{Eq:batch:estimator} and taking mathematical expectation. In order to show that the estimator is efficient we compute the Fisher information matrix corresponding to~\eqref{Eq:problem:measurement2}. To this end, we consider
$p(x_k\mid y_\ell,\,\ell\in\mathcal{L})$ -- the likelihood function of $x_k$ given the set of measurements $\set{y_\ell,\,\ell\in\mathcal{L}}$.
Recalling~\eqref{Eq:problem:measurement2} we note that the likelihood of $x_k$ given a single measurement $y_\ell$ is Gaussian with mean
%$H_\ell(A_{\ell,k}x_k+C_{\ell,k}u_{\ell,k})$
$H_\ell A_{\ell,k}x_k$
and covariance ${W}_{\ell,k}^{-T}R_\ell{W}_{\ell,k}^{-1}$. Since the measurement noise is white, the likelihood, given the set of measurements $\set{y_\ell,\,\ell\in\mathcal{L}}$, is given by the product
%\begin{align}\non
%&p(x_k\mid y_1,\ldots,y_{\size{\mathcal{L}}})\\\label{Eq:appendix:efficient:likelihood}
%&\quad=\prod_{\ell\in\mathcal{L}}\mathcal{N}(y_\ell;H_\ell(A_{\ell,k}x_k+C_{\ell,k}u_{\ell,k}),{W}_{\ell,k}^{-T}R_\ell{W}_{\ell,k}^{-1}),
%\end{align}
\begin{align}\label{Eq:appendix:efficient:likelihood}
&p(x_k\mid y_\ell,\,\ell\in\mathcal{L})
=\prod_{\ell\in\mathcal{L}}\mathcal{N}(y_\ell;H_\ell A_{\ell,k}x_k,{W}_{\ell,k}^{-T}R_\ell{W}_{\ell,k}^{-1}),
\end{align}
where $\mathcal{N}(y;\mu,\Sigma)$ is a Gaussian density function with mean $\mu$ and covariance matrix $\Sigma$ evaluated at $y$. The log-likelihood thus reads
%\begin{align}\non
%&\log p(x_k\mid y_1,\ldots,y_{\size{\mathcal{L}}})\\\label{Eq:appendix:efficient:loglikelihood}
%&\quad=C-\sum_{\ell\in\mathcal{L}}(H_\ell(A_{\ell,k}x_k+C_{\ell,k}u_{\ell,k})-y_\ell)^T\\
%&\qquad \times W_{\ell,k}R_\ell^{-1}W_{\ell,k}^T(H_\ell(A_{\ell,k}x_k+C_{\ell,k}u_{\ell,k})-y_\ell)
%\end{align}
\begin{align}\non
&\log p(x_k\mid y_\ell,\,\ell\in\mathcal{L})\\\label{Eq:appendix:efficient:loglikelihood}
&\quad=C-\sum_{\ell\in\mathcal{L}}(H_\ell A_{\ell,k}x_k-y_\ell)^TW_{\ell,k}R_\ell^{-1}W_{\ell,k}^T(H_\ell A_{\ell,k}x_k-y_\ell)
\end{align}
where $C$ is some constant that does not depend on $x_k$. Differentiating the latter twice with respect to $x_k$ yields, up to the minus sign, the inverse of~\eqref{theorem:covariance} meaning that the covariance of the estimator attains the Cram\'{e}r-Rao lower bound with equality rendering the estimator efficient.

\subsection{Proof of Lemma~\ref{lemma:scaling}}\label{appendix:scaling}
Suppose that the actual measurement noise covariance, $R_\ell$, is only known up to a constant factor $\alpha>0$ such that the value used in the algorithm is $\tilde{R}_\ell\triangleq\alpha{R}_\ell$. Plugging $\tilde{R}_\ell$ in~\eqref{Eq:batch:estimator}, it is readily seen that $\alpha$ cancels out, meaning that the imprecisely known covariance does not alter the estimator. This property is valid due to the lack of the process noise covariance term in the filter equation and cannot hold in the KF setup. We note that the covariance of the estimator, given in~\eqref{Eq:batch:covariance}, \emph{is} sensitive to the actual value of ${R}_\ell$.
